# Supplementary material for: ScreenAvoider: Protecting Computer Screens from Ubiquitous Cameras
Source: arXiv:1412.0008 source file (2014-11-28)
Supplement: Supplementary file 1 [file appendix.tex]

% !TEX root = main.tex

\subsection{Additional Figures}
\begin{figure}[htbp]
\begin{center}
\includegraphics[width=2in]{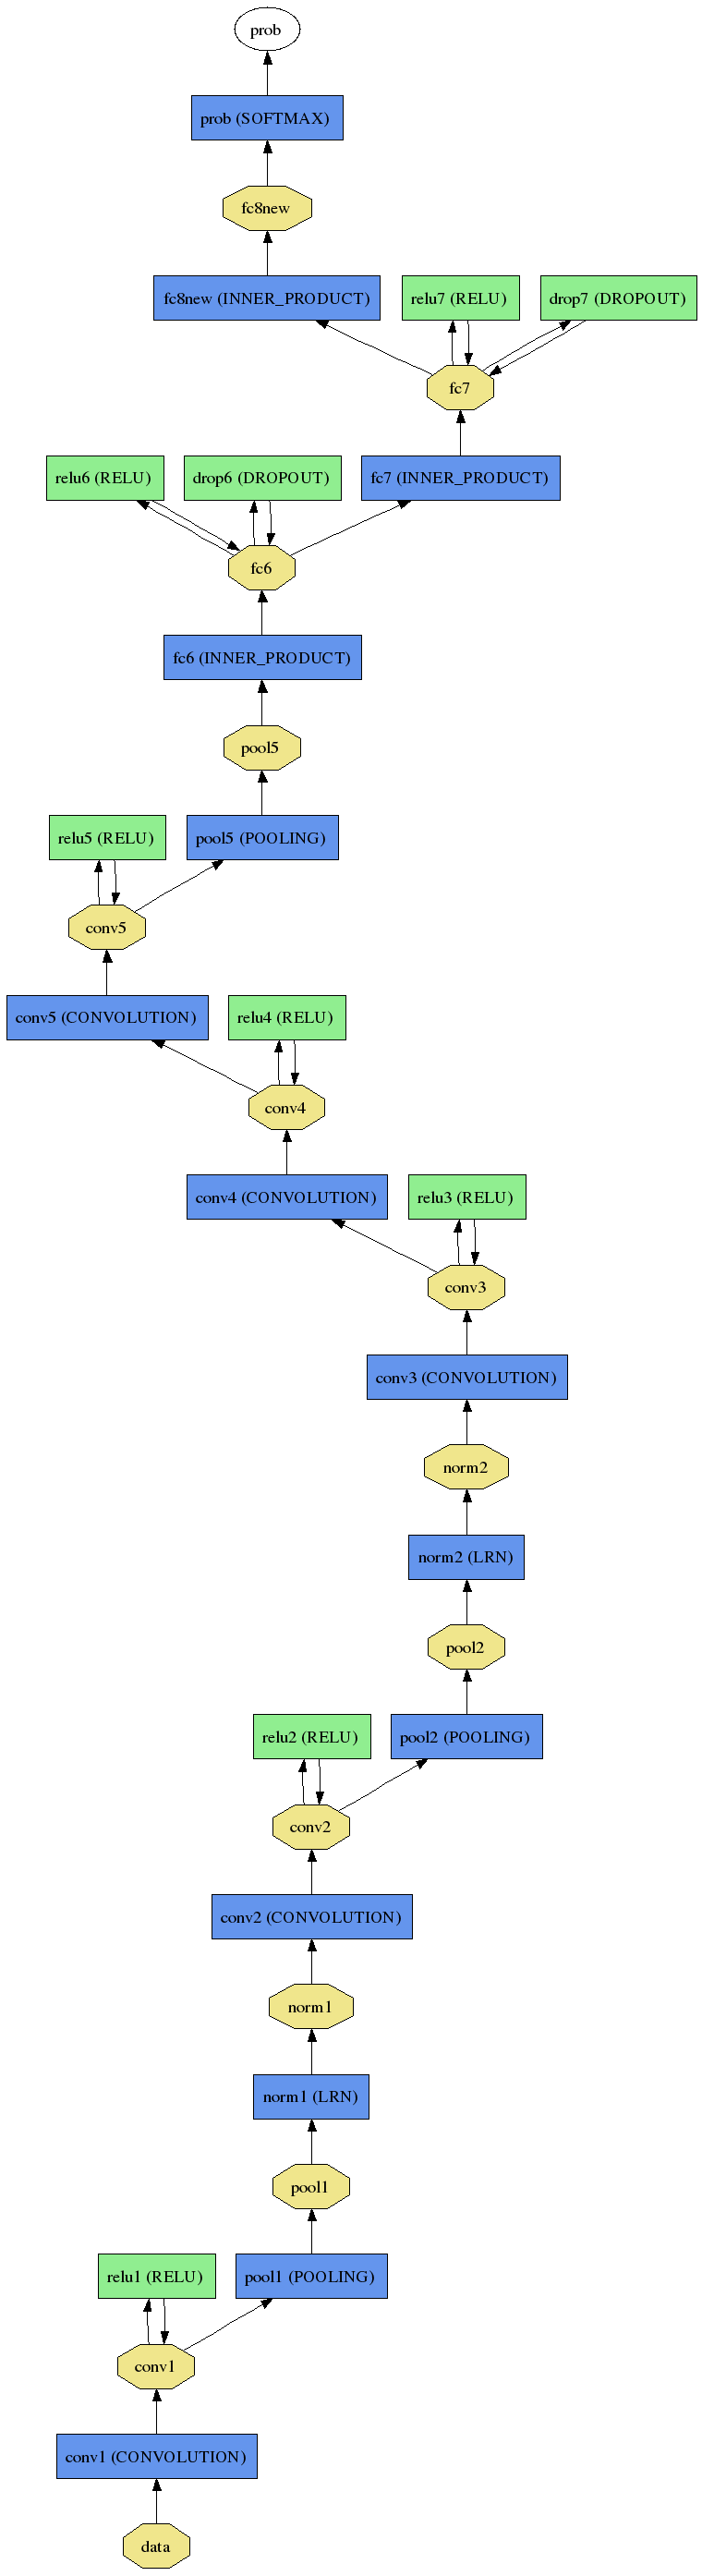}
\end{center}
\caption{A visualization of the classification network.}
\label{fig:network}
\end{figure}
